# Supplementary material for: First measurement of quasi-elastic $\Lambda$ baryon production in muon anti-neutrino interactions in the MicroBooNE detector
Source: arXiv:2212.07888 ancillary file (2023-06-09)
Supplement: Supplementary file 1 [file PRL_SM__Direct_Lambda_Production_in_MIcroBooNE.pdf]

# Supplemental Material: First measurement of quasi-elastic $\Lambda$ baryon production in muon anti-neutrino interactions in the MicroBooNE detector

## Kinematic Variables

After identifying a pair of tracks to form the candidate $\Lambda \to p + \pi^-$ decay, two kinematic variables are calculated: the invariant mass of the $\Lambda$ candidate, shown in Fig. 1a, and a quantity denoted as the angular deviation, shown in in Fig. 1b, the calculation of which is illustrated in Fig. 2.

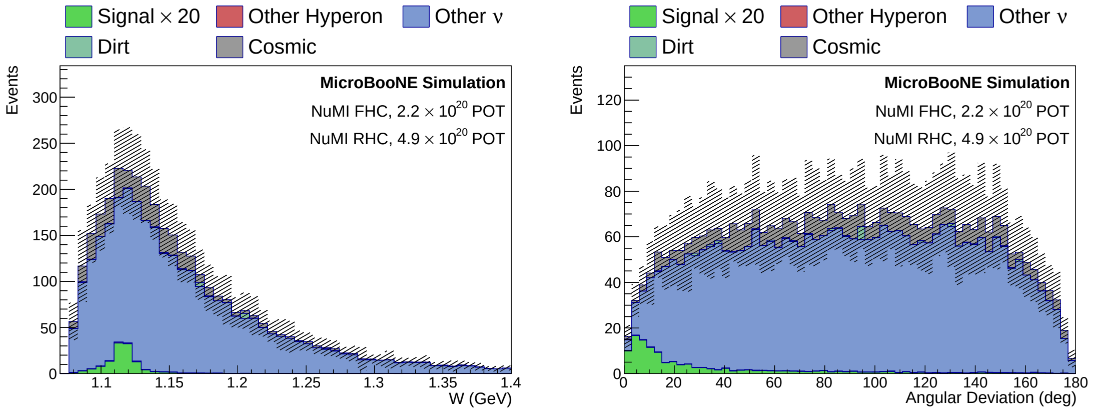


(a) Invariant mass.

(b) Angular deviation.

Figure 1: The kinematic variables employed by the event selection. The signal has been multiplied by 20 for visibility. The hatched regions indicate combined systematic and statistical uncertainties.

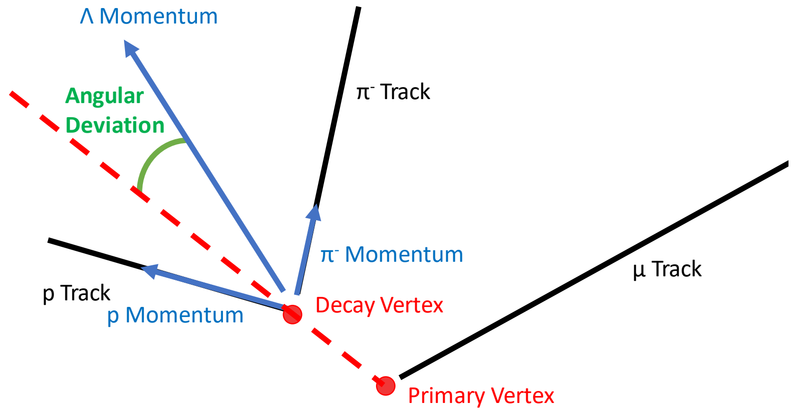


Figure 2: Calculation of the angular deviation variable.

## Partial Phase Space Definition

As the selection can only identify $\Lambda$ baryons that decay into a proton and $\pi^-$ with momenta above detection thresholds, the cross section must be corrected to only include this portion of the phase space. Our restricted phase space cross section, $\sigma_*$, is related to the total cross section for quasi-elastic $\Lambda$ production by:

$$\sigma_R = F\sigma, \tag{1}$$

$$F = \frac{1}{\sigma}\int_0^\infty f(p_\Lambda)\frac{d\sigma}{dp_\Lambda}dp_\Lambda. \tag{2}$$

$f(p_\Lambda)$ is the fraction of $\Lambda$ baryons decaying via $\Lambda \to p + \pi^-$ that will be above the detection thresholds. This function is shown in Fig. 3, and may be calculated with:

$$f(p_\Lambda) = \begin{cases} 0 & \text{if } A > B \\ \frac{B-A}{2} & \text{Otherwise} \end{cases}, \tag{3}$$

$$A = \max\left(\frac{\sqrt{M_p^2 + |p_p^{\text{thresh}}|^2} - \gamma E_p}{\beta\gamma p}, -1\right), \tag{4}$$

$$B = \min\left(\frac{-\sqrt{M_\pi^2 + |p_\pi^{\text{thresh}}|^2} + \gamma E_\pi}{\beta\gamma p}, 1\right), \tag{5}$$

$$E_p = \sqrt{M_p^2 + p^2}, \tag{6}$$

$$E_\pi = \sqrt{M_\pi^2 + p^2}. \tag{7}$$

$M_p$ and $M_\pi$ are the rest masses of the proton and $\pi^-$ respectively, $p_p^{\text{thresh}} = 0.3$ GeV, $p_\pi^{\text{thresh}} = 0.1$ GeV are the detection thresholds, $p = 0.101$ GeV is the momentum the decay products are emitted with in the $\Lambda$ baryon's rest frame, $\beta$ is the boost factor of the $\Lambda$ baryon in the detector's frame, and $\gamma = 1/\sqrt{1-\beta^2}$. Natural units are used.

Studying the selection efficiency as a function of the $\Lambda$ baryon's momentum, it is shown there is some shape to this distribution.

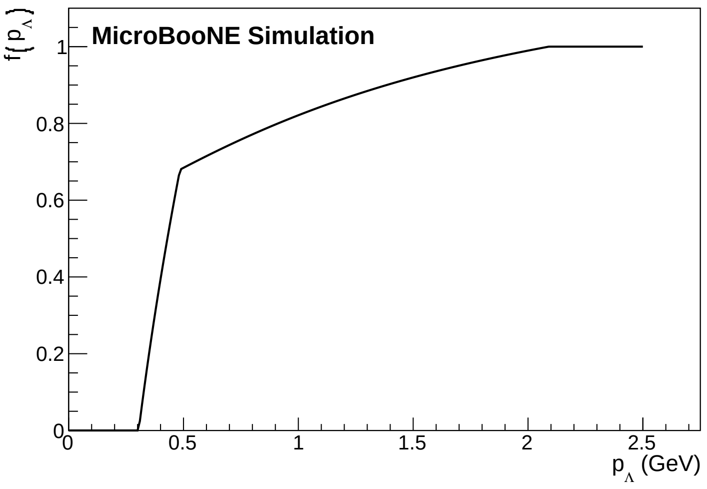


Figure 3: The function $f(p_\Lambda)$ featured in equations 2 and 3. The two discontinuities in gradient occur when one, and then both, particles produced in the decay are always above the detection threshold.

## Flux

Figure 4 displays the shape of the fluxes used in Monte Carlo simulations, including the combined neutrino mode (forward horn current, FHC) and anti-neutrino mode (reverse horn current, RHC) fluxes that corresponds to the data-taking period analyzed. The total $\bar{\nu}_\mu$ flux corresponding to the data analyzed is a sum of the FHC and RHC fluxes, and is recorded in Table 1. The total $\bar{\nu}_\mu$ flux is $4.43 \times 10^{15}$ m$^{-2}$, and the total number of targets in the fiducial volume is $6.53 \times 10^{29}$.

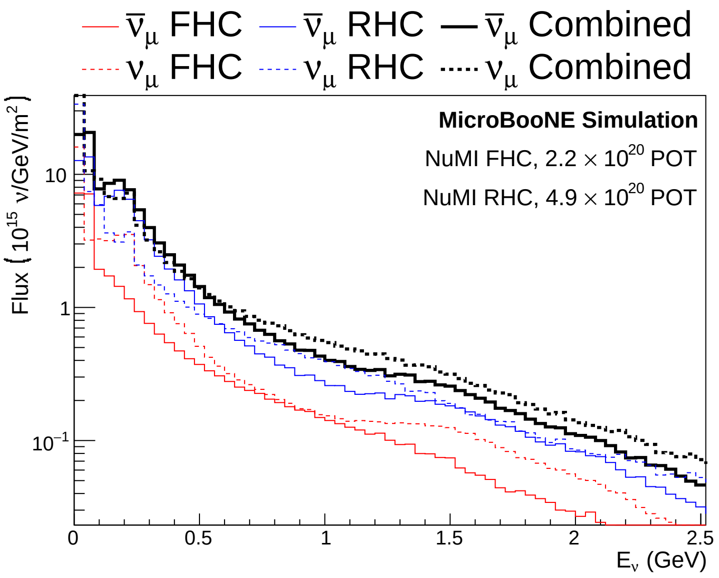


Figure 4: The neutrino and anti-neutrino fluxes corresponding to the data analyzed.

| Energy (GeV) | Prob. Dens. ($GeV^{-1}$) | Energy (GeV) | Prob. Dens. ($GeV^{-1}$) | Energy (GeV) | Prob Dens. ($GeV^{-1}$) |
|---|---|---|---|---|---|
| 0.02 | 4.500 | 1.70 | 0.039 | 3.38 | 0.005 |
| 0.06 | 4.663 | 1.74 | 0.038 | 3.42 | 0.004 |
| 0.10 | 1.756 | 1.78 | 0.036 | 3.46 | 0.004 |
| 0.14 | 1.934 | 1.82 | 0.033 | 3.50 | 0.004 |
| 0.18 | 2.040 | 1.86 | 0.030 | 3.54 | 0.004 |
| 0.22 | 1.730 | 1.90 | 0.029 | 3.58 | 0.004 |
| 0.26 | 1.223 | 1.94 | 0.028 | 3.62 | 0.003 |
| 0.30 | 0.899 | 1.98 | 0.025 | 3.66 | 0.004 |
| 0.34 | 0.689 | 2.02 | 0.025 | 3.70 | 0.003 |
| 0.38 | 0.562 | 2.06 | 0.024 | 3.74 | 0.003 |
| 0.42 | 0.470 | 2.10 | 0.023 | 3.78 | 0.003 |
| 0.46 | 0.394 | 2.14 | 0.021 | 3.82 | 0.003 |
| 0.50 | 0.324 | 2.18 | 0.019 | 3.86 | 0.003 |
| 0.54 | 0.268 | 2.22 | 0.017 | 3.90 | 0.003 |
| 0.58 | 0.238 | 2.26 | 0.017 | 3.94 | 0.003 |
| 0.62 | 0.209 | 2.30 | 0.015 | 3.98 | 0.003 |
| 0.66 | 0.185 | 2.34 | 0.015 | 4.02 | 0.003 |
| 0.70 | 0.170 | 2.38 | 0.014 | 4.06 | 0.003 |
| 0.74 | 0.152 | 2.42 | 0.012 | 4.10 | 0.003 |
| 0.78 | 0.142 | 2.46 | 0.011 | 4.14 | 0.002 |
| 0.82 | 0.127 | 2.50 | 0.010 | 4.18 | 0.002 |
| 0.86 | 0.120 | 2.54 | 0.009 | 4.22 | 0.002 |
| 0.90 | 0.108 | 2.58 | 0.009 | 4.26 | 0.002 |
| 0.94 | 0.107 | 2.62 | 0.009 | 4.30 | 0.002 |
| 0.98 | 0.097 | 2.66 | 0.009 | 4.34 | 0.002 |
| 1.02 | 0.090 | 2.70 | 0.008 | 4.38 | 0.002 |
| 1.06 | 0.089 | 2.74 | 0.008 | 4.42 | 0.002 |
| 1.10 | 0.081 | 2.78 | 0.008 | 4.46 | 0.002 |
| 1.14 | 0.077 | 2.82 | 0.008 | 4.50 | 0.002 |
| 1.18 | 0.076 | 2.86 | 0.008 | 4.54 | 0.002 |
| 1.22 | 0.077 | 2.90 | 0.007 | 4.58 | 0.002 |
| 1.26 | 0.069 | 2.94 | 0.007 | 4.62 | 0.002 |
| 1.30 | 0.071 | 2.98 | 0.006 | 4.66 | 0.001 |
| 1.34 | 0.070 | 3.02 | 0.006 | 4.70 | 0.001 |
| 1.38 | 0.063 | 3.06 | 0.006 | 4.74 | 0.001 |
| 1.42 | 0.063 | 3.10 | 0.006 | 4.78 | 0.001 |
| 1.46 | 0.059 | 3.14 | 0.006 | 4.82 | 0.001 |
| 1.50 | 0.058 | 3.18 | 0.005 | 4.86 | 0.001 |
| 1.54 | 0.054 | 3.22 | 0.005 | 4.90 | 0.001 |
| 1.58 | 0.050 | 3.26 | 0.005 | 4.94 | 0.001 |
| 1.62 | 0.047 | 3.30 | 0.005 | 4.98 | 0.001 |
| 1.66 | 0.044 | 3.34 | 0.005 | | |
| 1.70 | 0.039 | 3.38 | 0.005 | | |

Table 1: The $\bar{\nu}_\mu$ flux used in Monte Carlo simulations normalized to 1, in bins of 40 MeV, corresponding to a weighted average of FHC and RHC fluxes to describe the two data taking periods analyzed.

# Island Finding Algorithm

In order to determine if the $\Lambda$ candidate in the event forms a true secondary vertex, instead of analyzing the reconstructed tracks, the post-deconvolution wire activity is used, the raw form of which may be seen in Fig. 1 of the letter this material supports, and in Figs. 5a and 6a below. This may be interpreted as a grid, in which a single square has the dimensions of one channel by one time tick and stores the level of activity recorded on that wire at that time.

The first stage of the algorithm is to scan through every square in this grid and remove squares any with activity below a pre-defined threshold. Any squares above the threshold are all assigned a single value to indicate they are "occupied". The output of this stage is shown in Figs. 5b and 6b. The starting positions of the muon, proton, and pion tracks, transformed into channel-tick space, are used as "seeds" of islands, shown in cyan in Figs. 5c and 6c, and any neighboring squares that are occupied are added to their respective islands, and then the squares that neighbor those. This is done recursively until no new squares can be added. During this process, if any two islands meet, they will merge, and this merging is recorded. Fig. 5c shows two separate islands, with the muon island shown in blue, and the merged proton and pion in pink, while in Fig. 6c, all three islands merged. The passing condition is that the proton and pion islands must merge, while the muon remains separate. This process performed using the activity from each of the three wire planes separately, and events that pass this test in at least one plane are selected.

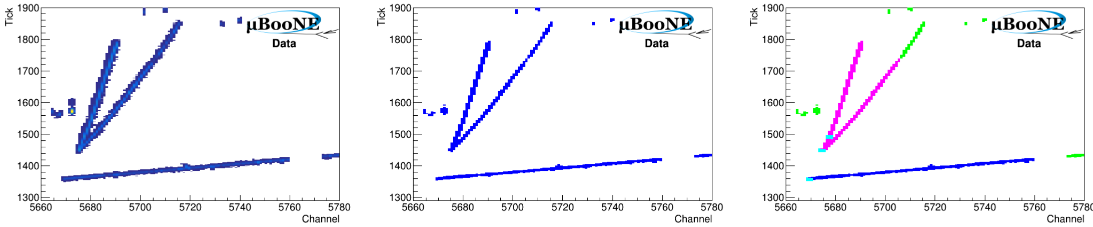


(a) Raw information. (b) After filtering. (c) After island creation.

Figure 5: The three stages of the island finding algorithm, shown for the event selected from the data in Fig. 1 of the letter. The blue and pink regions in panel 5c indicate the islands produced by the muon track and $\Lambda$ candidate respectively. The green regions correspond to wire activity not belonging to any either. The cyan squares show the starting positions of the three tracks when viewed from this wire plane.

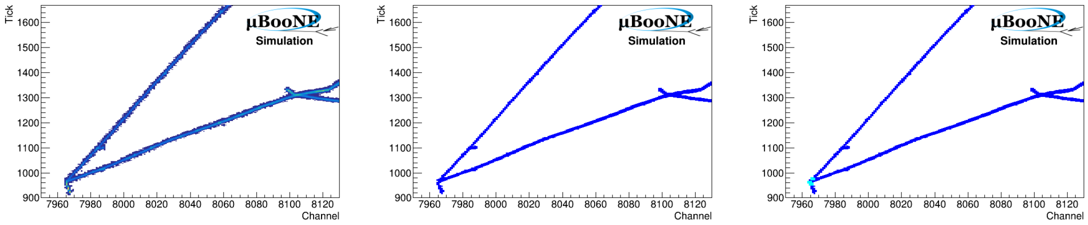


(a) Raw information. (b) After filtering. (c) After island creation.

Figure 6: The three stages of the island finding algorithm, shown for a Monte Carlo simulation event that failed this stage of the selection.

## Selection Efficiency Shape Dependence

The selection efficiency is known to exhibit some dependence on the shape of the differential cross section, due to irreducible detector effects such as the difficulty of reconstructing decays with opening angles close to 180°. Two approaches were explored to estimate the size of this effect and obtain a suitable uncertainty: varying the input parameters of neutrino event generators, and using the resulting changes in the shape of the differential cross section to reweight signal MC simulation events, and comparing the efficiencies obtained when applying the event selection to MC simulation samples produced with the GENIE and NuWro event generators. The model variations for the NuWro MC simulation shown in Fig. 7a were used to reweight the NuWro simulation sample, and the changes in the efficiency from the default NuWro simulation give possible uncertainties. Likewise, the variations in Fig. 7b were used to reweight the GENIE simulation sample, and the resulting estimates of the selection efficiency are compared to the value predicted by the default GENIE simulation.

Many combinations of settings for the NuWro and GENIE neutrino event generators were tested, and the cross section reweighted in terms of several variables, including the energy of the anti-neutrino, the squared four momentum transfer, and the momentum of the $\Lambda$ baryon. The largest change in efficiency was produced when varying the shape of the momentum distribution to simulate the effect of varying the hyperon-nucleus potentials, shown in Fig. 7a. This feature is only provided by the NuWro MC simulation, and so the resulting changes in efficiency were calculated by reweighting NuWro events simulated in the MicroBooNE cryostat, varying the strengths of the potentials between the extreme settings explored in Ref. [1]. The smallest and largest selection efficiencies obtained were 5.3% and 6.2%, compared with the efficiency of 5.5% for NuWro events when not applying the reweighting, suggesting a 16% uncertainty. The changes in shape of the differential cross section are illustrated in Fig. 7a. The axial mass parameter, $M_A$, was varied between 0.5 GeV and 2.0 GeV, shown for the GENIE generator in Fig. 7b. The resulting changes in efficiency are smaller than those of the hypernuclear potential variations. If efficiencies obtained from the two generators, on their default settings, are compared (6.8% versus 5.5%), an uncertainty of 19% is suggested; this is applied to be conservative.

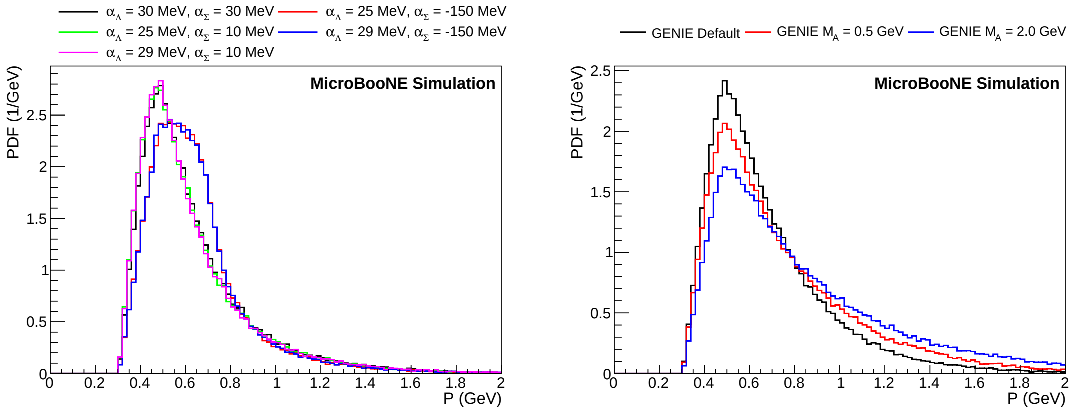


(a) Hypernuclear potential variations with NuWro.

(b) Axial mass variations with GENIE.

Figure 7: Generator model variations of the signal cross section, with different values of the hyperon axial mass and hyperon-nucleus potentials tested. The values of the $\Lambda$ nucleus and $\Sigma$ nucleus potentials in the current NuWro simulation samples used by MicroBooNE are $\alpha_\Lambda = 30$ MeV and $\alpha_\Sigma = 30$ MeV.

## Treatment of Hyperon Backgrounds

The event selection presented in the letter targets the CCQE-like $\Lambda$ production process, however several other mechanisms can produce $\Lambda$ and $\Sigma^0$ baryons, which constitute sources of background. In Table 1 of the letter, these are shared between the "Other $\Lambda$" and "Other hyperon" categories. These are not classified as part of the measured cross section, as the event selection yields very low acceptance rates of these events, for several reasons that are understood. Removing events producing electromagnetic showers removes a significant quantity of the $\Sigma^0$ baryons produced through the CCQE-like process, and these decay to photons, particles that create electromagnetic showers. The deep inelastic scattering and resonant backgrounds also often produce topologies with shower-like features, due to the high number of individual hadrons often created.

Imposing the same kinematic requirements on the decay of the $\Lambda$ baryons in these backgrounds as applied to the CCQE-like signal, and applying the automated selection only, the selection acceptances are as follows: 2.2% for the CCQE-like $\Sigma^0$ channel, 1.1% for the resonant channel, and 0.4% for the deep inelastic scattering process. These are in contrast with the 6.5% signal selection efficiency. Large systematic uncertainties are applied to the cross sections of these sources of background: a 100% uncertainty is applied to the CCQE-lile $\Sigma^0$ background, 35% to the RES $\Lambda$ background, and 25% to the DIS $\Lambda$ background. The overall systematic uncertainties on these three sources of background are approximately 110%, 65%, and 55% respectively. The total systematic uncertainty in the number of selected background events is around 60%.

# Sidebands

To confirm the background Monte Carlo simulation predictions are consistent with data, two sidebands are employed. The first, shown in Figs. 8a and 9a, is created by inverting the cut applied to the invariant mass, and the second, in Figs. 8b and 9b, by inverting the cut on the angular deviation. Data and MC predictions using both the NuMI beam, and the Booster Neutrino Beam (BNB) are compared. In the case of the NuMI data, the signal region is kept blind. The BNB data is expected to be extremely signal poor due to the low anti-neutrino flux produced by the beam, and the signal region is not kept blind, providing a check on the hyperon induced background. The Monte Carlo simulation predictions for the BNB do not include systematic uncertainties.

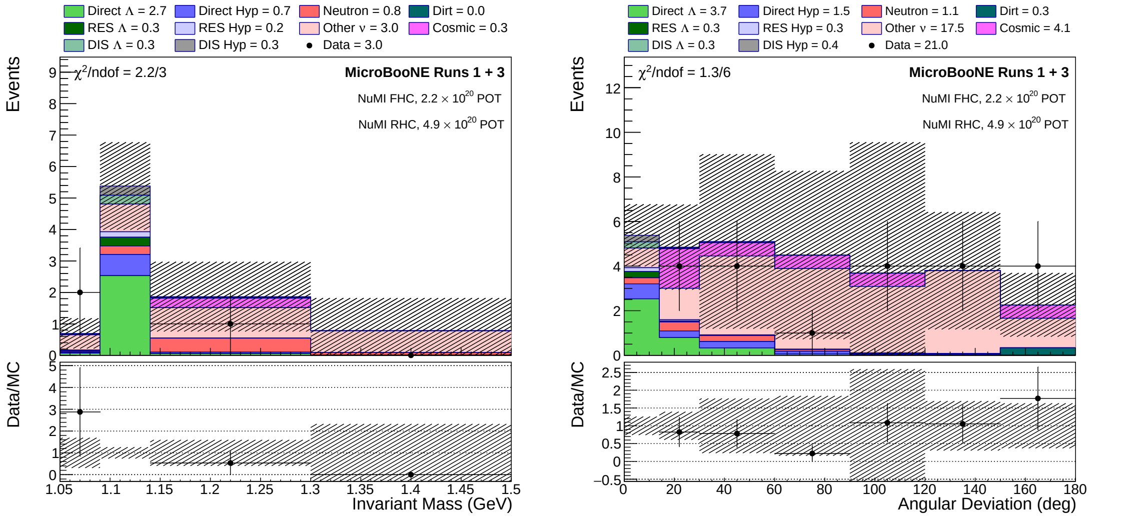


(a) Invariant mass.

(b) Angular deviation.

Figure 8: Sideband distributions constructed using NuMI data. The second bin of Fig. 8a and the first bin of Fig. 8b contain the signal and are kept blind. The large uncertainties are the result of low statistics in the alternative model samples used to estimate the uncertainties in the "other $\nu$" background, a problem avoided by the use of hand scanning in the primary result and the constraint procedure described in the next section.

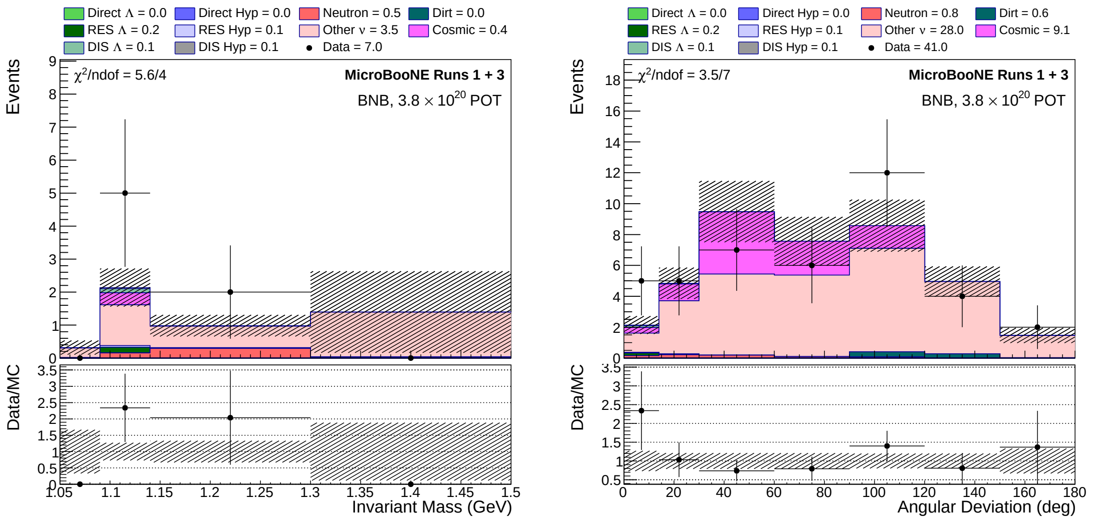


(a) Invariant mass.

(b) Angular deviation.

Figure 9: Sideband distributions constructed using BNB data.

## Constraint Procedure

The visual scan is employed to remove background containing reconstruction problems, for which the Monte Carlo simulation does not produce enough events to estimate the corresponding uncertainties in the signal region correctly. An alternative approach tested was to perform a constraint procedure using data passing the automated selection, but inverting the cuts applied to the angular deviation and invariant mass. This data, shown in Fig. 10, is split into two sets: a near sideband, containing events with angular deviations $< 50^\circ$ and $1.08 < W < 1.3$ GeV, and a far sideband, containing everything else.

A fit is then performed, varying the size of the bad-reconstruction background ("Other $\nu$" in Fig. 10), producing a new prediction shown in Fig. 10b. To obtain systematic uncertainties, we perform this fit in each systematic universe to obtain data-constrained sets of variations in the bad reconstruction background, which are then used to calculate the covariance between the flux, background, and efficiency. The extracted cross section is $1.8^{+2.0}_{-1.6} \times 10^{-40}$ cm$^2$/Ar; the Bayesian posterior distribution is presented in Fig. 11.

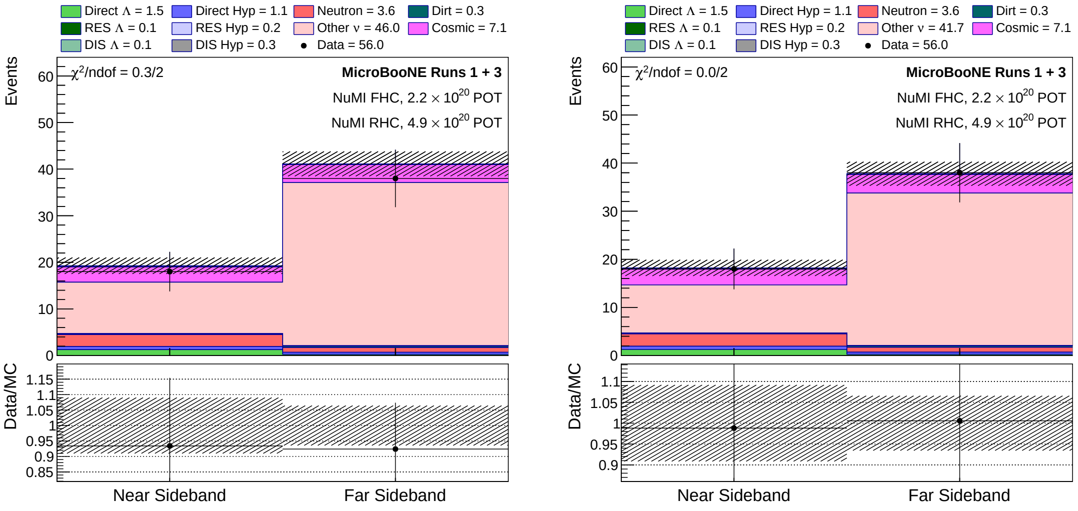


(a) Before fit. (b) After fit.

Figure 10: The data from the sideband compared with MC simulation before and after performing the fit.

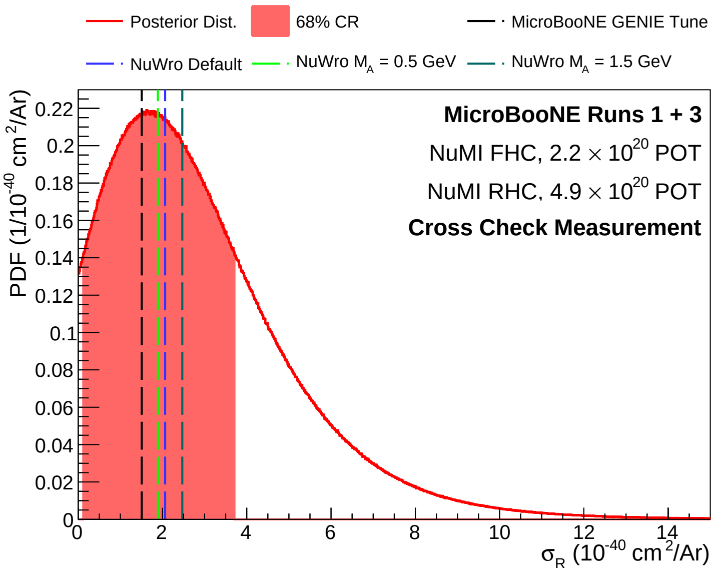


Figure 11: Bayesian posterior probability distribution of the extracted cross section obtained when employing the sideband constraint procedure.

## Selected Data

The five $\Lambda$ production candidates identified in the data by the automated selection are displayed below. The events selected from among these by each of the visual scanners are indicated in Table 2.

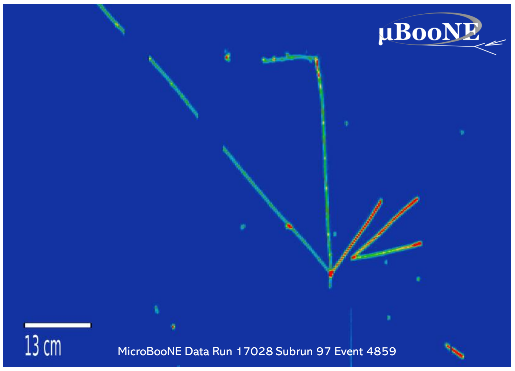


(a) Run 17028 subrun 97 event 4859.

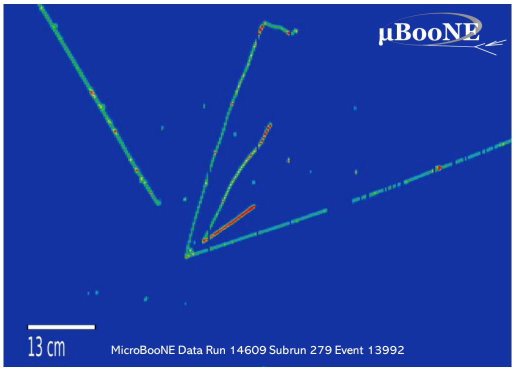


(b) Run 14609 subrun 279 event 13992.

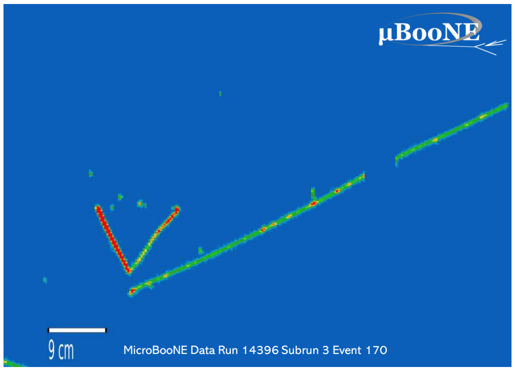


(c) Run 14396 subrun 3 event 170.

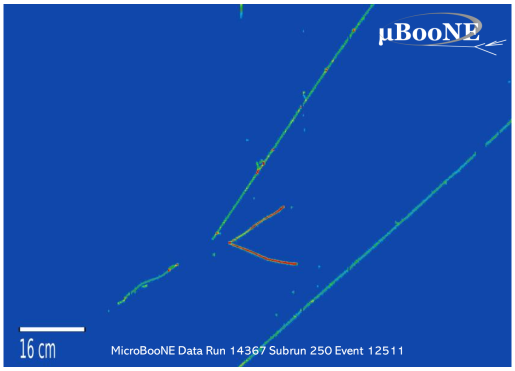


(d) Run 14367 subrun 250 event 12511.

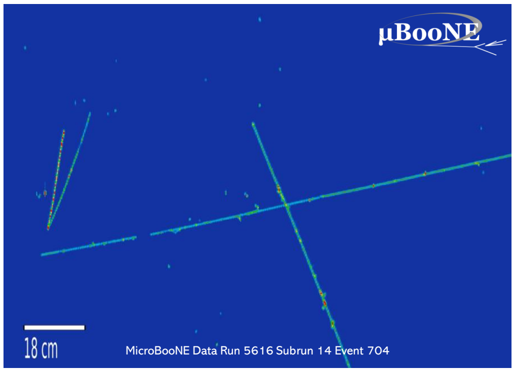


(e) Run 5616 subrun 14 event 704.

Figure 12: The $\Lambda$ candidates identified in the data by the automated selection.

| Run | Subrun | Event | Sc. 1 | Sc. 2 | Sc. 3 | Sc. 4 | Sc. 5 |
|---|---|---|---|---|---|---|---|
| 17028 | 97 | 4859 | | | ✓ | | ✓ |
| 14609 | 279 | 13992 | ✓ | | ✓ | | |
| 14396 | 3 | 170 | ✓ | ✓ | ✓ | ✓ | ✓ |
| 14367 | 250 | 12511 | ✓ | ✓ | ✓ | ✓ | ✓ |
| 5616 | 14 | 704 | ✓ | ✓ | ✓ | ✓ | ✓ |

Table 2: The events selected from the data by each of the five scanners.

# References

[1] C. Thorpe *et al.*, Second Class Currents, Axial Mass, and Nuclear Effects in Hyperon Production, Phys. Rev. C **104**, 035502 (2021).
